# Supplementary material for: Pair-production of the charged IDM scalars at high energy CLIC
Source: arXiv:2201.07146 source file (2022-07-01)
Supplement: Supplementary file 1 [file appendix.tex]

\section*{Appendix \label{appendix}}

    \begin{table}[htp]
        \begin{center}
        	\hspace*{3 cm}
            \caption{Benchmark points considered in study, accessible at  $e^+e^-$ colliders with $\mathcal{O}\left( \ensuremath\mathrm{TeV}\right)$ center-of-mass energies. $M_h=125.1\,\ensuremath\mathrm{GeV}$ for all points. BP21 and HP10 provide 100\% dark matter relic density \cite{Kalinowski:2018ylg}. \label{tab:bmhigh} }
            \begingroup
                \small
                
            	\setlength{\tabcolsep}{4pt}
                \include{tex/bp_params}
            \endgroup
        \end{center}
    \end{table}
